# Supplementary material for: CraftMesh: High-Fidelity Generative Mesh Manipulation via Poisson Seamless Fusion
Source: arXiv:2509.13688 source file (2026-03-29)
Supplement: Supplementary file 1 [file X_suppl.tex]

\clearpage
\setcounter{page}{1}
\maketitlesupplementary

\section{Title}
Text
